# Supplementary material for: Variational Approach for Job Shop Scheduling
Source: arXiv:2602.00408 ancillary file (2026-09-16)
Supplement: Supplementary file 1 [file supplementary.pdf]

# Supplementary Material

## A Transition based on Semi-active Schedule

In our paper, the transition is interpreted as a constructive procedure for generating a semi-active schedule. Each scheduling decision can be viewed as a single transition in our framework. In this decision, an operation is selected from available operations and starts immediately after the maximum completion time between its operation predecessor and earliest available time of its machine, thereby ensuring no unnecessary idle time. **Algorithm** 1 illustrates the constructive solution development process guided by a specified policy for a JSSP instance. Notably, these decision steps do not represent physical time in the JSSP context, but rather denote the sequential progression of operation selections within the semi-active schedule construction.

**Algorithm 1** Semi-active schedule construction based on policy $\pi$

**Input:** a JSSP instance and policy $\pi$
**Output:** $C_{\max}$ and schedule sequence
Initialize $\mathbf{m}_i, \mathbf{j}_j \leftarrow 0, \forall i \in \{1, \ldots, m\}, \forall j \in \{1, \ldots, n\}, C_{\max} \leftarrow 0$
Initialize empty sequence list $S \leftarrow []$
**for** $t = 0$ to length of solution sequence minus one **do**
    Select $O_{ij}$ by the policy $\pi(\cdot|s_t)$; $O_{ij} \in \mathcal{A}(s_t)$
    Append $O_{ij}$ to sequence $S$
    Let $\tilde{\mathbf{j}}_j \leftarrow \mathbf{j}_j$ for all $j$
    $\mathbf{m}_i \leftarrow \mathbf{m}_i + p_{ij}$
    $\mathbf{j}_j \leftarrow \mathbf{j}_j + p_{ij}$
    **if** $\mathbf{m}_i \leq \mathbf{j}_j$ **then**
        $\mathbf{m}_i \leftarrow \mathbf{j}_j$
    **else**
        $\mathbf{j}_j \leftarrow \mathbf{m}_i$
    **end if**
    $C_{\max} \leftarrow C_{\max} + \max \mathbf{j}_j - \max \tilde{\mathbf{j}}_j$
**end for**
**return** $C_{\max}, S$

## B Decoupling Representation and Policy via ELBO Maximization in JSSP

In DRL-based state-space approaches, JSSP state transitions are deterministic within a fixed problem instance. However, the requirement for generalizability across diverse JSSP instances introduces inevitable inter-instance variability and uncertainty. This uncertainty stems from the necessity to respond effectively to arbitrary, unknown problem instances. To interpret the inherent uncertainty of JSSP from a probabilistic perspective, we consider the distribution $p(G)$ from which JSSP instances are generated and the probability of achieving optimality $p(O = 1|G)$ given an instance $G$. Here, $O$ is a binary random variable where $O = 1$ denotes an optimal solution and $O = 0$ otherwise. Since our goal is to maximize the probability of achieving optimality during the instance generation process, we define the objective function $p(G, O = 1)$ as follows:

$$p(G, O = 1) = p(G) \cdot p(O = 1|G)$$

To marginalize $p(G, O = 1)$, we introduce a latent variable $z$ and an action sequence $a$ to define the joint distribution $p(G, O, z, a)$. By the chain rule, the objective is decomposed as follows:

$$p(G, O = 1) = \sum_{z,a} p(G, O, z, a) = \sum_{z,a} p(z) \cdot p(G|z) \cdot p(a|G, z) \cdot p(O = 1|G, z, a) \tag{1}$$

Here, $p(z)$ and $p(a|G, z)$ denote the latent prior and action prior, respectively, while $p(G|z)$ represents the instance likelihood and $p(O = 1|G, z, a)$ represents the optimality likelihood. The original objective, $p(G, O = 1)$, initially serves as a conceptual representation of the joint probability that a JSSP instance occurs and is solved optimally. Through marginalization, the physical meaning of this objective becomes clear: it describes a generative and evaluative sequence where a fundamental structural pattern $z$ exists ($p(z)$) , which is realized as a concrete instance $G$ ($p(G|z)$), followed by an action prior for that context ($p(a|G, z)$) , and finally the assessment of that action's optimality ($p(O = 1|G, z, a)$). Consequently, the abstract $p(G, O = 1)$ represents the integrated probability across all scenarios where a specific action is optimal for a given JSSP pattern. This decomposition provides each component with a distinct, interpretable probabilistic definition.

The optimality likelihood, $\max_a p(O = 1|G, z, a)$, provides a probabilistic representation of the objective to find the action sequence $a$ with the highest probability of being optimal for a given JSSP instance $G$ and latent variable $z$. We define $p(O = 1|G, z, a)$ as a distribution proportional to the exponentiated objective value $Q(z, a)$ of the action sequence: $p(O = 1|G, z, a) \propto \exp Q(z, a)$. Adopting an exponential distribution is a standard approach in maximum entropy reinforcement learning, such as soft Q-learning. This choice naturally satisfies the requirement for differentiability and ensures that the optimality probability approaches unity as $Q(z, a)$ is maximized. Furthermore, this formulation serves as the basis for decoupling the task into separate representation and control problems. We can thus express the lower bound for the log-likelihood of the objective function $p(G, O = 1)$ as follows:

$$\begin{aligned}
\log p(G, O) &= \log \sum_{z,a} [p(G, O, z, a) \cdot \frac{q(z, a|G)}{q(z, a|G)}] && (2)\\
&= \log \mathbb{E}_{z,a\sim q}[p(G, O, z, a) \cdot \frac{1}{q(z, a|G)}] && (3)\\
&\geq \mathbb{E}_{z,a\sim q}[\log p(G, O, z, a) - \log q(z, a|G)] && (4)\\
&= \mathbb{E}_{z,a\sim q}[\log p(G|z) + \log p(z) + \log p(a|G, z) + \log p(O|G, z, a) - \log q(z|G) - \log \pi(a|z, G)] && (5)\\
&= \mathbb{E}_{z,a\sim q}[\log p(G|z) + \log p(z) - \log q(z|G) + Q(z, a) - \log \pi(a|z, G) + p(a|G, z)] && (6)\\
&= \mathbb{E}_{z,a\sim q}[\log p(G|z)] - \mathrm{D_{KL}}[\log q(z|G)||p(z)] + \mathbb{E}_{z,a\sim q}[Q(z, a) - \log \pi(a|z, G) + \log p(a|G, z)] && (7)
\end{aligned}$$

Here, the posterior distribution $q(z, a|G)$ is factorized into the latent posterior $q(z|G)$ and the policy function $\pi(a|z, G)$, as shown in (8).

$$q(z, a|G) = q(z|G) \cdot \pi(a|z, G) \tag{8}$$

The equality in (2) marginalizes the objective function using the joint distribution $p(G, O, z, a)$ from a variational perspective. Equation (3) reformulates this as an expectation over the posterior distribution $q(z, a|G)$. By invoking Jensen's inequality, we obtain the lower bound in (4). This expression is further expanded in (6) by applying the definitions from (1) and (8). Finally, (7) decomposes the result into two distinct components: a representation learning term for the instance, $\mathbb{E}_{z\sim q}[\log p(G|z)] - D_{KL}[q(z|G) \parallel p(z)]$, and a policy learning term, $\mathbb{E}_{z,a\sim q}[Q(z, a) - \log \pi(a|z, G) + \log p(a|G, z)]$. Thus, maximizing the ELBO effectively decouples the original objective into two complementary tasks: representation learning and policy optimization.

## C Maximum Entropy Policy Optimization

Assuming a uniform prior for $p(a|G,z)$—given that the optimal action is unknown a priori—$\log p(a|G,z)$ can be treated as a constant. Consequently, the policy term $\mathcal{J}(\theta)$ defined in (7) can be expressed in the form of maximum entropy reinforcement learning (RL) with a baseline $V(z)$ for the policy $\pi_\theta$ as follows:

$$J(\pi_\theta) = \mathbb{E}_{z\sim q}\mathbb{E}_{a\sim\pi}[Q(z,a) - V(z) - \log \pi_\theta(a|z,G)] \tag{9}$$

Methods for solving maximum entropy RL problems, such as Soft Actor-Critic (SAC) [1] and soft Q-learning [2], have primarily been developed within the framework of continuous control. These approaches typically utilize the reparameterization trick; however, its application is inherently limited in discrete action settings such as JSSP [3]. While [4] attempted to apply maximum entropy RL to JSSP by computing expectations over all possible discrete actions, such an approach becomes computationally intractable as the action space expands with the increasing number of machines and jobs.

To circumvent these challenges, we approach the maximum entropy RL problem from the perspective of Policy Gradient (PG) with entropy regularization. This approach is justified by the equivalence between Soft Policy Iteration (SPI) and maximum entropy RL (i.e., (9)), as detailed in the proof below. Notably, since SPI provides an optimality guarantee, the derived Policy Gradient method also inherits theoretically sound convergence properties.

Specifically, by treating the state value function $\exp V(z)$ as the partition function $Z(z)$, maximizing (9) is essentially equivalent to the minimization problem in (11). Furthermore, (10) describes the soft policy improvement process within SPI for JSSP instances encountered randomly in the latent space.

$$\theta^* = \arg\min_\theta \tilde{D}(\pi_\theta) \tag{10}$$

$$\tilde{D}(\pi_\theta) = \mathbb{E}_{z\sim q}[\mathrm{D}_{\mathrm{KL}}[\pi_\theta(\cdot|z)||\exp Q(z,a)/Z(z)]] \tag{11}$$

*Proof.* Expanding the KL divergence term, we obtain:

$$\begin{aligned} &D_{KL}[\pi_\theta(\cdot|z)||\exp Q(z,\cdot)/Z(z)] \\ &= \mathbb{E}_{a\sim\pi_\theta}[\log \pi_\theta(a|z) - Q(z,a) + \log Z(z)] \end{aligned} \tag{12}$$

Given the relationship $V(z) = \log Z(z)$ in the maximum entropy RL framework, it follows that:

$$\begin{aligned} &D_{KL}[\pi_\theta(\cdot|z)||\exp Q(z,\cdot)/Z(z)] \\ &= \mathbb{E}_{a\sim\pi_\theta}[\log \pi_\theta(a|z) - Q(z,a)] + V(z) \end{aligned} \tag{13}$$

Thus:

$$\begin{aligned} &- D_{KL}[\pi_\theta(\cdot|z)||\exp Q(z,\cdot)/Z(z)] \\ &= \mathbb{E}_{a\sim\pi_\theta}[Q(z,a) - V(z) - \log \pi_\theta(a|z)] \end{aligned} \tag{14}$$

$J(\pi_\theta) = -\tilde{D}(\pi_\theta)$ holds true. □

# D Hyperparameter Details

To identify the optimal hyperparameter settings, we conducted a grid search by defining 6 base configurations (IDs 1–6) and evaluating each under five different values of $E_r \in \{20000, 40000, 60000, 80000, 100000\}$. This resulted in a total of 30 unique hyperparameter combinations. The initial learning rate was fixed at $1.0 \times 10^{-4}$ for all settings.

Table 1: Base hyperparameter configurations for grid search. Each configuration was evaluated for five different $E_r$ values. All $\mathrm{MLP}$ layers in these configurations employ the ELU activation function.

| ID | 1 | 2 | 3 | 4 | 5 | 6 |
|---|---|---|---|---|---|---|
| $\alpha_{\text{APPNP}}$ | 0.10 | 0.05 | 0.05 | 0.05 | 0.05 | 0.05 |
| $d_{\text{latent}}$ | 108 | 96 | 128 | 96 | 90 | 98 |
| $d_{\text{glimpse}}$ | 36 | 32 | 32 | 32 | 36 | 30 |
| $d_{\text{logit}}$ | 48 | 54 | 54 | 54 | 64 | 56 |
| $d_{\text{graph}}$ | 96 | 96 | 96 | 96 | 92 | 86 |
| $M_{\text{head}}$ | 2 | 1 | 1 | 1 | 2 | 1 |
| $\mathrm{MLP}_{\text{aggr}}$ | [128, 96] | [196, 128] | [196, 96] | [196, 128] | [196, 128] | [196, 144] |
| $\alpha_{\text{ent}}$ (init) | $5 \times 10^{-4}$ | $1 \times 10^{-3}$ | $1 \times 10^{-5}$ | 0.0 | $1 \times 10^{-4}$ | $1 \times 10^{-4}$ |
| $\alpha_{\text{ent}}$ (min) | 0.0 | 0.0 | $1 \times 10^{-6}$ | 0.0 | 0.0 | 0.0 |
| LR Decay (rate) | 0.95 | 0.99 | 0.99 | 1.00 | 0.995 | 0.995 |
| LR Decay (step) | 500 | 600 | 1000 | - | 600 | 500 |
| Min LR | $5.0 \times 10^{-5}$ | $5.0 \times 10^{-5}$ | $5.0 \times 10^{-5}$ | $5.0 \times 10^{-5}$ | $5.0 \times 10^{-5}$ | $7.5 \times 10^{-5}$ |

Table 2: Common Hyperparameters and Model Architectures

| Hyperparameter | Value / Structure |
|---|---|
| Initial Learning Rate | $1.0 \times 10^{-4}$ |
| Max Nodes ($N_*$) | 100 |
| $\mathrm{MLP}_{\text{shared}}$ Structure | [256, 256], ELU activation |
| $\mathrm{MLP}_{\mu}$ Structure | [256, 256], ELU activation |
| $\mathrm{MLP}_{\sigma}$ Structure | [256, 256], ELU activation |
| Critic network ($V(z)$) | [128, 64, 32, 16, 1], ELU activation |
| Glimpse iterations ($L$) | 3 |
| Normalization | Batch Normalization (1D) |

Table 3: Sequence of upsampling layers to reach sequence length $N_*^2 = 10,000$.

| Layer | Configuration | Output Dimension |
|---|---|---|
| Input Layer | Linear Projection | $512 \times 1$ |
| Upsampling 1 | $\mathrm{ConvTr1d}(512, 256)$ | $256 \times L_1$ |
| Upsampling 2 | $\mathrm{ConvTr1d}(256, 128)$ | $128 \times L_2$ |
| Upsampling 3 | $\mathrm{ConvTr1d}(128, 64)$ | $64 \times L_3$ |
| Iterative Block | $\mathrm{ConvTr1d}(64, 64)$ | $64 \times L \geq N_*^2$ |

The generative model $g_\psi(z)$ reconstructs the graph structure and node features from a latent vector $z \in \mathbb{R}^{d_{\text{latent}}}$. For $N_* = 100$, the architecture begins by mapping the latent vector via a linear projection to a $512$-dimensional space, which is then followed by a series of 1D Transposed Convolutions characterized by a kernel size of $k = 4$, a stride of $s = 2$, and padding of $p = 1$. Each of these upsampling stages incorporates Batch Normalization and ReLU activation functions to progressively refine the representation throughout the reconstruction process. From the features generated by the final upsampling block, two separate heads branch out to predict edge and node information:

**Edge Probability ($P_{\text{edge}}$):** Generates adjacency information via point-wise convolution:

$$P_{\text{edge}} = \sigma\left(\text{Conv1d}_{k=1}(64 \to d_{\text{edge\_types}})\right)$$

**Node Probability ($P_{\text{node}}$):** Extracts features for exactly $N_* = 100$ nodes using adaptive pooling:

$$P_{\text{node}} = \sigma\left(\text{Conv1d}_{k=1}(\text{AdaptiveAvgPool1d}(100))\right)$$

# E Test Results

Table 4: Test Results for Taillard's Datasets

| Dataset | Size | UB | Zhang [A] | Park [A] | Park [B] | Yuan | Oh | V2GS |
|---|---|---|---|---|---|---|---|---|
| TA01 | 15 × 15 | 1231 | 1443 | **1389** | 1452 | 1494 | 1472 | 1422 |
| TA02 | 15 × 15 | 1244 | 1544 | 1519 | 1411 | 1603 | 1417 | **1382** |
| TA03 | 15 × 15 | 1218 | 1440 | 1457 | 1396 | 1409 | 1409 | **1369** |
| TA04 | 15 × 15 | 1175 | 1637 | 1465 | 1348 | 1508 | **1330** | 1409 |
| TA05 | 15 × 15 | 1224 | 1619 | 1352 | 1382 | 1563 | **1333** | 1376 |
| TA06 | 15 × 15 | 1238 | 1601 | 1481 | 1413 | 1437 | **1364** | 1424 |
| TA07 | 15 × 15 | 1227 | 1568 | 1554 | 1380 | 1439 | 1397 | **1372** |
| TA08 | 15 × 15 | 1217 | 1468 | 1488 | **1374** | 1472 | 1422 | 1461 |
| TA09 | 15 × 15 | 1274 | 1627 | 1556 | 1523 | 1531 | 1527 | **1516** |
| TA10 | 15 × 15 | 1241 | 1527 | 1501 | 1493 | 1449 | **1427** | 1481 |
| TA11 | 20 × 15 | 1357 | 1794 | 1626 | 1612 | 1668 | 1622 | **1555** |
| TA12 | 20 × 15 | 1367 | 1805 | 1668 | 1600 | 1656 | **1559** | 1576 |
| TA13 | 20 × 15 | 1343 | 1932 | 1715 | 1625 | 1670 | 1626 | **1585** |
| TA14 | 20 × 15 | 1345 | 1664 | 1642 | 1590 | 1718 | 1526 | **1503** |
| TA15 | 20 × 15 | 1339 | 1730 | 1672 | 1676 | 1716 | **1600** | **1600** |
| TA16 | 20 × 15 | 1360 | 1710 | 1700 | 1550 | 1656 | 1538 | **1520** |
| TA17 | 20 × 15 | 1462 | 1897 | 1678 | 1753 | 1761 | **1677** | 1682 |
| TA18 | 20 × 15 | 1396 | 1794 | 1684 | 1668 | 1675 | 1676 | **1628** |
| TA19 | 20 × 15 | 1332 | 1682 | 1900 | 1622 | 1599 | 1564 | **1525** |
| TA20 | 20 × 15 | 1348 | 1739 | 1752 | 1604 | 1582 | **1523** | 1582 |
| TA21 | 20 × 20 | 1642 | 2252 | 2199 | 1921 | 1933 | 1969 | **1849** |
| TA22 | 20 × 20 | 1600 | 2102 | 2049 | 1844 | 1963 | 1877 | **1840** |
| TA23 | 20 × 20 | 1557 | 2085 | 2006 | 1879 | 1846 | **1831** | 1932 |
| TA24 | 20 × 20 | 1644 | 2200 | 2020 | 1922 | 1940 | 1853 | **1828** |
| TA25 | 20 × 20 | 1595 | 2201 | 1981 | 1897 | 1999 | **1809** | 1821 |
| TA26 | 20 × 20 | 1643 | 2176 | 2057 | 1887 | 1948 | 1986 | **1861** |
| TA27 | 20 × 20 | 1680 | 2132 | 2187 | 2009 | 2068 | **1924** | 1960 |
| TA28 | 20 × 20 | 1603 | 2146 | 2054 | 1813 | 1895 | **1773** | 1935 |
| TA29 | 20 × 20 | 1625 | 1952 | 2210 | **1875** | 1947 | 1935 | 1912 |
| TA30 | 20 × 20 | 1584 | 2035 | 2140 | 1913 | 2015 | 1914 | **1864** |
| TA31 | 30 × 15 | 1764 | 2565 | 2251 | **2055** | 2122 | 2162 | 2142 |
| TA32 | 30 × 15 | 1784 | 2388 | 2378 | 2268 | 2270 | **2163** | 2244 |
| TA33 | 30 × 15 | 1791 | 2324 | 2316 | 2281 | 2446 | **2206** | 2218 |
| TA34 | 30 × 15 | 1828 | 2332 | 2319 | **2061** | 2180 | 2143 | 2120 |
| TA35 | 30 × 15 | 2007 | 2505 | 2333 | 2218 | 2254 | 2173 | **2149** |
| TA36 | 30 × 15 | 1819 | 2497 | 2210 | 2154 | 2262 | 2231 | **2117** |
| TA37 | 30 × 15 | 1771 | 2325 | 2201 | **2112** | 2183 | 2170 | 2146 |
| TA38 | 30 × 15 | 1673 | 2302 | 2151 | 1970 | 2129 | **1925** | 2109 |
| TA39 | 30 × 15 | 1795 | 2410 | 2138 | 2146 | 2128 | 2100 | **2011** |
| TA40 | 30 × 15 | 1669 | 2140 | **2007** | 2030 | 2064 | 2019 | 2046 |

| Dataset | Size | UB | Zhang [A] | Park [A] | Park [B] | Yuan | Oh | V2GS |
|---|---|---|---|---|---|---|---|---|
| TA41 | 30 × 20 | 2005 | 2667 | 2654 | 2572 | 2559 | **2419** | 2464 |
| TA42 | 30 × 20 | 1937 | 2664 | 2579 | 2397 | 2416 | 2337 | **2267** |
| TA43 | 30 × 20 | 1846 | 2431 | 2737 | 2310 | 2358 | **2261** | 2280 |
| TA44 | 30 × 20 | 1979 | 2714 | 2772 | 2456 | 2517 | 2425 | **2410** |
| TA45 | 30 × 20 | 2000 | 2637 | 2435 | 2445 | 2550 | 2291 | **2239** |
| TA46 | 30 × 20 | 2006 | 2776 | 2681 | 2541 | 2612 | **2375** | 2407 |
| TA47 | 30 × 20 | 1889 | 2476 | 2428 | 2280 | 2352 | **2214** | 2273 |
| TA48 | 30 × 20 | 1937 | 2490 | 2440 | 2358 | 2413 | **2272** | 2420 |
| TA49 | 30 × 20 | 1961 | 2556 | 2446 | **2301** | 2380 | 2359 | 2428 |
| TA50 | 30 × 20 | 1923 | 2628 | 2530 | 2453 | 2458 | 2363 | **2330** |
| TA51 | 50 × 15 | 2760 | 3599 | **3145** | 3382 | 3488 | 3332 | 3244 |
| TA52 | 50 × 15 | 2756 | 3341 | 3157 | 3231 | 3334 | 3185 | **3103** |
| TA53 | 50 × 15 | 2717 | 3106 | 3103 | 3083 | 3044 | 3045 | **3017** |
| TA54 | 50 × 15 | 2839 | 3266 | 3278 | 3068 | 3191 | 3002 | **2924** |
| TA55 | 50 × 15 | 2679 | 3232 | 3142 | **3078** | 3230 | 3138 | 3098 |
| TA56 | 50 × 15 | 2781 | 3378 | 3258 | **3065** | 3122 | 3100 | 3116 |
| TA57 | 50 × 15 | 2943 | 3471 | 3230 | 3266 | 3254 | 3279 | **3188** |
| TA58 | 50 × 15 | 2885 | 3454 | 3469 | 3321 | 3404 | 3273 | **3164** |
| TA59 | 50 × 15 | 2655 | 3381 | 3108 | 3044 | 3102 | 3043 | **2976** |
| TA60 | 50 × 15 | 2723 | 3281 | 3256 | 3036 | 3004 | 3030 | **3003** |
| TA61 | 50 × 20 | 2868 | 3654 | 3425 | **3202** | 3434 | 3213 | 3241 |
| TA62 | 50 × 20 | 2869 | 3617 | 3626 | 3339 | 3471 | 3358 | **3327** |
| TA63 | 50 × 20 | 2755 | 3397 | 3110 | 3118 | 3120 | **3067** | 3188 |
| TA64 | 50 × 20 | 2702 | 3275 | 3329 | **2989** | 3133 | 3002 | 2991 |
| TA65 | 50 × 20 | 2725 | 3359 | 3339 | **3168** | 3394 | 3204 | 3239 |
| TA66 | 50 × 20 | 2845 | 3388 | 3340 | 3199 | 3232 | 3186 | **3158** |
| TA67 | 50 × 20 | 2825 | 3567 | 3371 | 3236 | 3397 | 3215 | **3210** |
| TA68 | 50 × 20 | 2784 | 3514 | 3265 | 3072 | 3219 | **3059** | 3100 |
| TA69 | 50 × 20 | 3071 | 3592 | 3798 | 3535 | 3560 | 3470 | **3351** |
| TA70 | 50 × 20 | 2995 | 3643 | 3919 | 3436 | 3480 | 3430 | **3379** |
| TA71 | 100 × 20 | 5464 | 6452 | 5962 | 5879 | 5960 | **5823** | 5850 |
| TA72 | 100 × 20 | 5181 | 5695 | 5522 | **5456** | 5543 | 5498 | 5500 |
| TA73 | 100 × 20 | 5568 | 6411 | 6335 | **6052** | 6206 | 6130 | 6113 |
| TA74 | 100 × 20 | 5339 | 5885 | 5827 | **5513** | 5741 | 5596 | 5626 |
| TA75 | 100 × 20 | 5392 | 6355 | 6042 | 5992 | 6201 | 5936 | **5814** |
| TA76 | 100 × 20 | 5342 | 6135 | **5707** | 5773 | 5906 | 5896 | 5759 |
| TA77 | 100 × 20 | 5436 | 6056 | 5737 | **5637** | 5725 | 5739 | 5695 |
| TA78 | 100 × 20 | 5394 | 6101 | 5979 | 5833 | 5767 | 5771 | **5722** |
| TA79 | 100 × 20 | 5358 | 5943 | 5799 | **5556** | 5819 | 5664 | **5556** |
| TA80 | 100 × 20 | 5183 | 5892 | 5718 | 5545 | 5582 | **5460** | 5550 |

Table 5: Test Results for Demirkol's Datasets

| Dataset | Size | UB | Zhang [A] | Yuan | Oh | Zhang [B] | V2GS |
|---|---|---|---|---|---|---|---|
| DMU01 | 20 × 15 | 2563 | 3323 | 3304 | 3048 | 3247 | **3003** |
| DMU02 | 20 × 15 | 2706 | 3630 | 3425 | 3315 | 3431 | **3182** |
| DMU03 | 20 × 15 | 2731 | 3660 | 3202 | 3189 | 3573 | **3171** |
| DMU04 | 20 × 15 | 2669 | 3816 | 3229 | 3141 | 3399 | **3022** |
| DMU05 | 20 × 15 | 2749 | 3897 | 3381 | 3303 | 3604 | **3190** |
| DMU41 | 20 × 15 | 3248 | 4316 | 4336 | 4308 | 4367 | **4003** |
| DMU42 | 20 × 15 | 3390 | 4858 | 4351 | 4145 | 4846 | **4097** |
| DMU43 | 20 × 15 | 3441 | 4887 | **4328** | 4370 | 4690 | 4382 |
| DMU44 | 20 × 15 | 3488 | 5151 | 4681 | **4279** | 4822 | 4386 |
| DMU45 | 20 × 15 | 3272 | 4615 | 4544 | 4278 | 4597 | **3954** |
| DMU06 | 20 × 20 | 3244 | 4358 | 3956 | **3612** | 4109 | 3690 |
| DMU07 | 20 × 20 | 3046 | 3671 | 3574 | **3489** | 3901 | 3514 |
| DMU08 | 20 × 20 | 3188 | 4048 | 3867 | **3696** | 3821 | 3818 |
| DMU09 | 20 × 20 | 3092 | 4482 | 3774 | **3575** | 3775 | **3575** |
| DMU10 | 20 × 20 | 2984 | 4021 | 3518 | **3336** | 3704 | 3360 |
| DMU46 | 20 × 20 | 4035 | 5876 | **4989** | 5160 | 5330 | 5024 |
| DMU47 | 20 × 20 | 3939 | 5771 | 4955 | **4861** | 5120 | 5063 |
| DMU48 | 20 × 20 | 3763 | 5034 | 4785 | **4513** | 4929 | 4596 |
| DMU49 | 20 × 20 | 3710 | 5470 | 4897 | 4562 | 5152 | **4471** |
| DMU50 | 20 × 20 | 3729 | 5314 | 4716 | **4615** | 4884 | 4709 |
| DMU11 | 30 × 15 | 3430 | 4435 | 4404 | 4288 | 4378 | **4134** |
| DMU12 | 30 × 15 | 3495 | 4864 | 4203 | **4082** | 4485 | 4364 |
| DMU13 | 30 × 15 | 3681 | 4918 | 4949 | 4491 | 4893 | **4333** |
| DMU14 | 30 × 15 | 3394 | 4130 | 4104 | **3814** | 4199 | 3994 |
| DMU15 | 30 × 15 | 3343 | 4392 | 4213 | **4085** | 4194 | 4141 |
| DMU51 | 30 × 15 | 4167 | 6241 | 5521 | 5711 | 6395 | **5251** |
| DMU52 | 30 × 15 | 4311 | 6714 | 5608 | 6093 | 6485 | **5444** |
| DMU53 | 30 × 15 | 4394 | 6724 | 5906 | 5860 | 6665 | **5331** |
| DMU54 | 30 × 15 | 4362 | 6522 | **5519** | 5775 | 6341 | 5606 |
| DMU55 | 30 × 15 | 4271 | 6639 | 5698 | 5888 | 6123 | **5331** |
| DMU16 | 30 × 20 | 3751 | 4953 | 4500 | **4344** | 4897 | 4395 |
| DMU17 | 30 × 20 | 3814 | 5379 | 4716 | **4443** | 5026 | 4463 |
| DMU18 | 30 × 20 | 3844 | 5100 | 4708 | 4561 | 4822 | **4549** |
| DMU19 | 30 × 20 | 3768 | 4889 | 4953 | 4534 | 4727 | **4363** |
| DMU20 | 30 × 20 | 3710 | 4859 | 4530 | **4331** | 4799 | 4423 |
| DMU56 | 30 × 20 | 4941 | 7328 | **6439** | 6508 | 6918 | 6528 |
| DMU57 | 30 × 20 | 4655 | 6704 | **6072** | 6229 | 6738 | 6507 |
| DMU58 | 30 × 20 | 4708 | 6721 | 6577 | 6174 | 6672 | **5854** |
| DMU59 | 30 × 20 | 4624 | 7109 | 6420 | 6617 | 6722 | **6048** |
| DMU60 | 30 × 20 | 4755 | 6632 | 6332 | 6547 | 6752 | **5971** |

| Dataset | Size | UB | Zhang [A] | Yuan | Oh | Zhang [B] | V2GS |
|---|---|---|---|---|---|---|---|
| DMU21 | 40 × 15 | 4380 | 5317 | 5444 | 5418 | 5235 | **5010** |
| DMU22 | 40 × 15 | 4725 | 5534 | 5483 | **5151** | 5482 | 5162 |
| DMU23 | 40 × 15 | 4668 | 5620 | 5238 | 5068 | 5298 | **5067** |
| DMU24 | 40 × 15 | 4648 | 5479 | 5148 | 5096 | 5443 | **4949** |
| DMU25 | 40 × 15 | 4164 | 4775 | 5557 | **4584** | 4832 | **4584** |
| DMU61 | 40 × 15 | 5172 | 8053 | 6918 | 7310 | 8005 | **6661** |
| DMU62 | 40 × 15 | 5265 | 8091 | 6777 | 7383 | 7907 | **6635** |
| DMU63 | 40 × 15 | 5326 | 8031 | **6907** | 7775 | 7984 | 7074 |
| DMU64 | 40 × 15 | 5250 | 7738 | 6751 | 7257 | 7914 | **6612** |
| DMU65 | 40 × 15 | 5190 | 7577 | **7040** | 7347 | 7793 | 7154 |
| DMU26 | 40 × 20 | 4647 | 5908 | 5591 | **5422** | 5913 | 5464 |
| DMU27 | 40 × 20 | 4848 | 6418 | 5980 | 5845 | 5925 | **5652** |
| DMU28 | 40 × 20 | 4692 | 5986 | 5831 | **5345** | 5799 | 5525 |
| DMU29 | 40 × 20 | 4691 | 6051 | 6268 | **5367** | 5946 | 5619 |
| DMU30 | 40 × 20 | 4732 | 5988 | 5759 | 5606 | 5855 | **5456** |
| DMU66 | 40 × 20 | 5717 | 8475 | 8107 | 8319 | 8607 | **8016** |
| DMU67 | 40 × 20 | 5813 | 8791 | 8246 | **7932** | 8622 | 7936 |
| DMU68 | 40 × 20 | 5773 | 8693 | 8286 | 8205 | 8560 | **7647** |
| DMU69 | 40 × 20 | 5709 | 8634 | 7780 | 7844 | 8566 | **7720** |
| DMU70 | 40 × 20 | 5889 | 8601 | 8123 | 8085 | 8465 | **7970** |
| DMU31 | 50 × 15 | 5640 | 7156 | 6765 | 6281 | 6845 | **6214** |
| DMU32 | 50 × 15 | 5927 | 6506 | 6005 | **5940** | 6369 | 5967 |
| DMU33 | 50 × 15 | 5728 | 6192 | 6915 | 6049 | 6122 | **5925** |
| DMU34 | 50 × 15 | 5385 | 6257 | 6138 | 5678 | 6096 | **5657** |
| DMU35 | 50 × 15 | 5635 | 6302 | 7057 | 6015 | 6135 | **5995** |
| DMU71 | 50 × 15 | 6233 | 9797 | 8353 | 8924 | 9628 | **8083** |
| DMU72 | 50 × 15 | 6483 | 9926 | 8516 | 9598 | 9512 | **8428** |
| DMU73 | 50 × 15 | 6163 | 9933 | 8440 | 8862 | 9753 | **8213** |
| DMU74 | 50 × 15 | 6220 | 9833 | 8662 | 9272 | 9639 | **8076** |
| DMU75 | 50 × 15 | 6197 | 9892 | **7858** | 8926 | 9573 | 8235 |
| DMU36 | 50 × 20 | 5621 | 7213 | 6763 | **6589** | 6886 | 6723 |
| DMU37 | 50 × 20 | 5851 | 7296 | 7213 | 6854 | 7075 | **6728** |
| DMU38 | 50 × 20 | 5713 | 7410 | 7421 | **6697** | 7361 | 6851 |
| DMU39 | 50 × 20 | 5747 | 6827 | 6608 | 6428 | 6690 | **6236** |
| DMU40 | 50 × 20 | 5577 | 7325 | 7184 | 6571 | 7042 | **6535** |
| DMU76 | 50 × 20 | 6813 | 9698 | 10014 | 9689 | 10157 | **9410** |
| DMU77 | 50 × 20 | 6822 | 10693 | 9848 | 9890 | 10185 | **9357** |
| DMU78 | 50 × 20 | 6770 | 9986 | 9604 | 9505 | 10298 | **9404** |
| DMU79 | 50 × 20 | 6970 | 10936 | 9902 | 10336 | 10767 | **9883** |
| DMU80 | 50 × 20 | 6686 | 9875 | 9473 | 9478 | 9934 | **8773** |

Table 6: Test Results for Lawrance's Datasets

| Dataset | Size | UB | Park [A] | Park [B] | Yuan | Oh | V2GS |
|---|---|---|---|---|---|---|---|
| LA01 | 10 × 5 | 666 | 805 | 680 | **670** | 708 | 718 |
| LA02 | 10 × 5 | 655 | **687** | 768 | 756 | 738 | 732 |
| LA03 | 10 × 5 | 597 | 862 | 734 | 736 | **650** | 677 |
| LA04 | 10 × 5 | 590 | 650 | 698 | 796 | 664 | **641** |
| LA05 | 10 × 5 | 593 | **593** | **593** | **593** | 648 | 650 |
| LA06 | 15 × 5 | 926 | **926** | **926** | **926** | **926** | **926** |
| LA07 | 15 × 5 | 890 | 931 | 1008 | 1041 | **922** | 931 |
| LA08 | 15 × 5 | 863 | **863** | **863** | 996 | 876 | 917 |
| LA09 | 15 × 5 | 951 | **951** | **951** | 985 | **951** | 962 |
| LA10 | 15 × 5 | 958 | 966 | **958** | 974 | **958** | 1002 |
| LA11 | 20 × 5 | 1222 | 1276 | 1254 | 1228 | **1222** | 1238 |
| LA12 | 20 × 5 | 1039 | **1039** | **1039** | 1050 | 1052 | 1042 |
| LA13 | 20 × 5 | 1150 | **1150** | **1150** | **1150** | **1150** | 1156 |
| LA14 | 20 × 5 | 1292 | **1292** | **1292** | **1292** | **1292** | 1308 |
| LA15 | 20 × 5 | 1207 | 1282 | 1395 | 1477 | 1371 | **1275** |
| LA16 | 10 × 10 | 945 | 1134 | **1047** | 1051 | 1109 | 1091 |
| LA17 | 10 × 10 | 784 | 953 | 888 | 857 | **841** | 866 |
| LA18 | 10 × 10 | 848 | 1049 | 947 | 947 | 935 | **893** |
| LA19 | 10 × 10 | 842 | **880** | 963 | 979 | 899 | 908 |
| LA20 | 10 × 10 | 902 | 1042 | 989 | 990 | 977 | **935** |
| LA21 | 15 × 10 | 1046 | 1309 | 1261 | **1179** | 1208 | 1227 |
| LA22 | 15 × 10 | 927 | 1158 | 1027 | 1057 | **997** | 1059 |
| LA23 | 15 × 10 | 1032 | **1085** | 1145 | 1145 | 1124 | 1134 |
| LA24 | 15 × 10 | 935 | 1129 | 1088 | 1074 | **1059** | 1106 |
| LA25 | 15 × 10 | 977 | 1308 | 1117 | 1099 | **1082** | 1176 |
| LA26 | 20 × 10 | 1218 | 1553 | 1458 | 1383 | **1376** | 1484 |
| LA27 | 20 × 10 | 1235 | 1624 | 1516 | 1515 | 1453 | **1448** |
| LA28 | 20 × 10 | 1216 | 1438 | **1357** | 1451 | 1428 | 1437 |
| LA29 | 20 × 10 | 1152 | 1582 | **1320** | 1389 | 1347 | 1494 |
| LA30 | 20 × 10 | 1355 | 1649 | 1490 | 1477 | **1414** | 1444 |
| LA31 | 30 × 10 | 1784 | **1817** | 1906 | 1916 | 1903 | 1857 |
| LA32 | 30 × 10 | 1850 | 1977 | **1850** | 1969 | 1895 | 1972 |
| LA33 | 30 × 10 | 1719 | 1795 | 1731 | 1881 | 1745 | **1719** |
| LA34 | 30 × 10 | 1721 | 1895 | 1784 | 1846 | **1756** | 1827 |
| LA35 | 30 × 10 | 1888 | 2041 | 1969 | 2059 | 1990 | **1964** |
| LA36 | 15 × 15 | 1268 | 1489 | 1449 | 1426 | **1372** | 1418 |
| LA37 | 15 × 15 | 1397 | 1623 | 1653 | 1649 | **1552** | 1596 |
| LA38 | 15 × 15 | 1196 | 1421 | 1444 | 1398 | **1373** | 1455 |
| LA39 | 15 × 15 | 1233 | 1555 | 1430 | 1469 | 1386 | **1376** |
| LA40 | 15 × 15 | 1222 | 1570 | 1357 | 1400 | **1322** | 1355 |

Table 7: Test Results for SWV, ABZ, ORB, FT and YN Datasets

| Dataset | Size | UB | Park [A] | Park [B] | Yuan | Oh | V2GS |
|---|---|---|---|---|---|---|---|
| SWV01 | $20 \times 10$ | 1407 | 1761 | 1913 | 1882 | 1810 | **1697** |
| SWV02 | $20 \times 10$ | 1475 | 1846 | 1998 | 1856 | 1831 | **1688** |
| SWV03 | $20 \times 10$ | 1398 | 1892 | 1830 | 1912 | 1773 | **1677** |
| SWV04 | $20 \times 10$ | 1464 | 1908 | 1971 | 1935 | 1948 | **1788** |
| SWV05 | $20 \times 10$ | 1424 | **1796** | 1922 | 1831 | 1833 | 1820 |
| SWV06 | $20 \times 15$ | 1671 | **2068** | 2216 | 2257 | 2160 | 2106 |
| SWV07 | $20 \times 15$ | 1594 | 2194 | 2037 | 2012 | 1964 | **1870** |
| SWV08 | $20 \times 15$ | 1752 | **2191** | 2255 | 2219 | 2344 | 2354 |
| SWV09 | $20 \times 15$ | 1655 | 2278 | 2196 | 2272 | **2136** | 2189 |
| SWV10 | $20 \times 15$ | 1743 | 2141 | 2279 | 2252 | 2342 | **2119** |
| SWV11 | $50 \times 10$ | 2983 | 3989 | 4390 | 3642 | 4082 | **3604** |
| SWV12 | $50 \times 10$ | 2977 | 4136 | 4532 | **3648** | 4279 | 3656 |
| SWV13 | $50 \times 10$ | 3104 | 4008 | 4602 | 3926 | 4460 | **3917** |
| SWV14 | $50 \times 10$ | 2968 | 3758 | 4387 | **3519** | 4060 | 3551 |
| SWV15 | $50 \times 10$ | 2885 | 3860 | 4402 | **3652** | 4077 | 3698 |
| SWV16 | $50 \times 10$ | 2924 | **2924** | **2924** | 3125 | **2924** | 2958 |
| SWV17 | $50 \times 10$ | 2794 | 2840 | **2794** | 2987 | **2794** | 2803 |
| SWV18 | $50 \times 10$ | 2852 | **2852** | **2852** | 3081 | 2859 | 2881 |
| SWV19 | $50 \times 10$ | 2843 | 2961 | 2992 | **2903** | 2959 | 2905 |
| SWV20 | $50 \times 10$ | 2823 | **2823** | **2823** | 2845 | 2826 | 2840 |
| ABZ05 | $10 \times 10$ | 1234 | 1353 | 1336 | 1360 | **1334** | 1343 |
| ABZ06 | $10 \times 10$ | 943 | 1043 | 981 | **980** | 997 | 1032 |
| ABZ07 | $20 \times 15$ | 656 | 887 | 791 | **767** | 768 | **767** |
| ABZ08 | $20 \times 15$ | 665 | 843 | 787 | 805 | 789 | **756** |
| ABZ09 | $20 \times 15$ | 678 | 848 | **832** | 874 | **832** | 855 |
| ORB01 | $10 \times 10$ | 1059 | 1336 | 1276 | 1318 | **1253** | 1281 |
| ORB02 | $10 \times 10$ | 888 | 1067 | **958** | 1068 | 963 | **958** |
| ORB03 | $10 \times 10$ | 1005 | **1202** | 1335 | 1212 | 1220 | 1298 |
| ORB04 | $10 \times 10$ | 1005 | 1281 | 1178 | 1144 | 1224 | **1132** |
| ORB05 | $10 \times 10$ | 887 | 1082 | **1042** | 1147 | 1103 | 1068 |
| ORB06 | $10 \times 10$ | 1010 | **1178** | 1222 | 1283 | 1273 | 1224 |
| ORB07 | $10 \times 10$ | 397 | 477 | **456** | 473 | 471 | 472 |
| ORB08 | $10 \times 10$ | 899 | 1156 | 1178 | 1186 | **983** | 1031 |
| ORB09 | $10 \times 10$ | 934 | 1143 | 1145 | 1123 | **1107** | 1141 |
| ORB10 | $10 \times 10$ | 944 | 1087 | 1080 | 1171 | **1046** | 1061 |
| FT06 | $6 \times 6$ | 55 | 71 | 59 | 60 | **56** | 59 |
| FT10 | $10 \times 10$ | 930 | 1142 | 1111 | 1102 | **1038** | 1060 |
| FT20 | $20 \times 5$ | 1165 | 1338 | 1498 | 1332 | **1260** | 1302 |
| YN01 | $20 \times 20$ | 884 | 1118 | 1027 | 1020 | 1031 | **1008** |
| YN02 | $20 \times 20$ | 904 | 1097 | 1037 | 1070 | **1034** | 1036 |
| YN03 | $20 \times 20$ | 892 | 1083 | 1046 | 1073 | 1014 | **999** |
| YN04 | $20 \times 20$ | 968 | 1258 | 1216 | 1230 | 1205 | **1189** |

## F Flowshop Index

The **flow shop index** ($0 \leq I_f \leq 1$) is introduced as a metric to quantify the prevalence of consistent job sequences within a job shop environment. For any machine pair $(i, k)$, let $n_{ik}$ represent the count of jobs that are processed on machine $i$ and subsequently transferred to machine $k$ for the next operation (with $n_{ik} = 0$ if $i = k$). The flow shop index for a specific machine pair is defined as:

$$I_f^{ik} = \frac{\max(n_{ik} - 1, 0)}{n - 1} \tag{15}$$

The cumulative flow shop index for the system is then expressed as:

$$I_f = \frac{1}{m - 1} \sum_{i=1}^{n} \sum_{k=1}^{n} I_f^{ik} \tag{16}$$

Furthermore, to account for the problem scale, the **scaled flow shop index** is defined as follows:

$$I_{scaled} = \frac{I_f}{\log(n \times m)} \tag{17}$$

# References


[1] T. Haarnoja, H. Tang, P. Abbeel, and S. Levine, "Reinforcement learning with deep energy-based policies," in *International conference on machine learning*. PMLR, 2017, pp. 1352–1361.

[2] T. Haarnoja, A. Zhou, P. Abbeel, and S. Levine, "Soft actor-critic: Off-policy maximum entropy deep reinforcement learning with a stochastic actor," in *International conference on machine learning*. Pmlr, 2018, pp. 1861–1870.

[3] P. Christodoulou, "Soft actor-critic for discrete action settings," *arXiv preprint arXiv:1910.07207*, 2019.

[4] W. Zhang, F. Zhao, C. Yang, C. Du, X. Feng, Y. Zhang, Z. Peng, and X. Mei, "A novel soft actor–critic framework with disjunctive graph embedding and autoencoder mechanism for job shop scheduling problems," *Journal of Manufacturing Systems*, vol. 76, pp. 614–626, 2024.
